# Supplementary material for: Anomalous propagators and the particle-particle channel: Hedin's equations
Source: arXiv:2406.07062 ancillary file (2024-09-04)
Supplement: Supplementary file 1 [file si.pdf]

# Supplemental Material for "Anomalous propagators and the particle-particle channel: Hedin's equations"


Antoine Marie,[1,*] Pina Romaniello,[2,3] and Pierre-François Loos[1,†]

[1] *Laboratoire de Chimie et Physique Quantiques (UMR 5626), Université de Toulouse, CNRS, UPS, France*

[2] *Laboratoire de Physique Théorique, Université de Toulouse, CNRS, UPS, France*

[3] *European Theoretical Spectroscopy Facility (ETSF)*


This document contains additional details on the derivation of the particle-particle (pp) version of Hedin's equations. Missing notations can be found in the main manuscript. Section I deals with the derivation of the Schwinger relation for an external pairing potential. In Sec. II, we derive the equation of motion (EOM) for the Gorkov propagator. Section III reports a closed set of equations for this propagator in terms of the Coulomb operator. In Sec. IV, we present the so-called pp Gorkov-Hedin equations, while Sec. V gathers the analog of Hedin's equations for the pp channel. Finally, we discuss vertex corrections in Sec. VI.

## I. THE SCHWINGER RELATION

This section aims at deriving Eq. (13) of the main manuscript [see Eq. (11) below] which is a Schwinger relation for pairing response [1]. The Hamiltonian of the system in the presence of an external pairing potential is

$$\begin{aligned}\hat{H}'(t) &= \hat{H} + \hat{\mathcal{U}}(t)\\ &= \int \mathrm{d}(\mathbf{x}_1\mathbf{x}_{1'})\, \hat{\psi}^\dagger(\mathbf{x}_1) h(\mathbf{x}_1\mathbf{x}_{1'})\hat{\psi}(\mathbf{x}_{1'}) + \frac{1}{2}\iint \mathrm{d}(\mathbf{x}_1\mathbf{x}_2\mathbf{x}_{1'}\mathbf{x}_{2'})\, \hat{\psi}^\dagger(\mathbf{x}_1)\hat{\psi}^\dagger(\mathbf{x}_2) v(\mathbf{x}_1\mathbf{x}_2;\mathbf{x}_{1'}\mathbf{x}_{2'})\hat{\psi}(\mathbf{x}_{2'})\hat{\psi}(\mathbf{x}_{1'})\\ &+ \frac{1}{2}\left[\int \mathrm{d}(\mathbf{x}_1\mathbf{x}_{1'})\, \hat{\psi}(\mathbf{x}_1) U^{\text{hh}}(\mathbf{x}_1\mathbf{x}_{1'};t)\hat{\psi}(\mathbf{x}_{1'}) + \int \mathrm{d}(\mathbf{x}_1\mathbf{x}_{1'})\, \hat{\psi}^\dagger(\mathbf{x}_1) U^{\text{ee}}(\mathbf{x}_1\mathbf{x}_{1'};t)\hat{\psi}^\dagger(\mathbf{x}_{1'})\right],\end{aligned} \tag{1}$$

where $h$ is the one-body Hamiltonian, $v$ is the two-body Coulomb interaction, while $U^{\text{hh}}$ and $U^{\text{ee}}$ are the external pairing potentials. The external potential is assumed to be Hermitian, i.e. $\hat{\mathcal{U}}^\dagger(t) = \hat{\mathcal{U}}(t)$, which implies that

$$U^{\text{hh}}(\mathbf{x}_1\mathbf{x}_{1'};t) = [U^{\text{ee}}(\mathbf{x}_{1'}\mathbf{x}_1;t)]^*, \tag{2}$$

and to fulfill the following limiting conditions

$$\lim_{t\to\pm\infty} U^{\text{hh}}(\mathbf{x}_1\mathbf{x}_{1'};t) = 0, \qquad \lim_{t\to\pm\infty} U^{\text{ee}}(\mathbf{x}_1\mathbf{x}_{1'};t) = 0. \tag{3}$$

Finally, the external pairing potentials are assumed to be anti-symmetric with respect to their two spatial coordinates, that is,

$$U^{\text{hh}}(\mathbf{x}_{1'}\mathbf{x}_1;t) = -U^{\text{hh}}(\mathbf{x}_1\mathbf{x}_{1'};t), \qquad U^{\text{ee}}(\mathbf{x}_{1'}\mathbf{x}_1;t) = -U^{\text{ee}}(\mathbf{x}_1\mathbf{x}_{1'};t). \tag{4}$$

The next step is to differentiate the anomalous Green's functions with respect to the external potential. The expression of the Heisenberg picture operators given in the main manuscript [see Eqs. (4a) and (4b)] relied on the assumption that $\hat{H}$ is time-independent. However, this is not the case in the presence of $\hat{\mathcal{U}}(t)$ and the Heisenberg picture of the field operators is

$$\hat{\psi}(1) = \hat{U}^\dagger_{\hat{H}'}(t_1)\hat{\psi}(\mathbf{x}_1)\hat{U}_{\hat{H}'}(t_1), \qquad \hat{\psi}^\dagger(1) = \hat{U}^\dagger_{\hat{H}'}(t_1)\hat{\psi}^\dagger(\mathbf{x}_1)\hat{U}_{\hat{H}'}(t_1), \tag{5}$$

where $\hat{U}_{\hat{H}'}$ is the time-evolution operator corresponding to the time-dependent Hamiltonian $\hat{H}'(t)$. These expressions cannot be easily differentiated with respect to $U^{\text{ee}}$ and $U^{\text{hh}}$.

Expressing the Green's function in terms of interaction picture operators

$$\hat{\psi}_{\text{I}}(1) = e^{\text{i}\hat{H}t_1}\hat{\psi}(\mathbf{x}_1)e^{-\text{i}\hat{H}t_1}, \qquad \hat{\psi}^\dagger_{\text{I}}(1) = e^{\text{i}\hat{H}t_1}\hat{\psi}^\dagger(\mathbf{x}_1)e^{-\text{i}\hat{H}t_1}. \tag{6}$$


* amarie@irsamc.ups-tlse.fr

† loos@irsamc.ups-tlse.fr

is better suited for this purpose. The corresponding expressions for the anomalous propagators are (see Appendix B of Ref. 2)

$$G^{\text{hh}}(11';[U]) = \frac{\langle\Psi_0|\hat{T}\left[\hat{S}\hat{\psi}_{\text{I}}(1)\hat{\psi}_{\text{I}}(1')\right]|\Psi_0\rangle}{\langle\Psi_0|\hat{S}|\Psi_0\rangle}, \qquad G^{\text{ee}}(11';[U]) = \frac{\langle\Psi_0|\hat{T}\left[\hat{S}\hat{\psi}_{\text{I}}^{\dagger}(1)\hat{\psi}_{\text{I}}^{\dagger}(1')\right]|\Psi_0\rangle}{\langle\Psi_0|\hat{S}|\Psi_0\rangle}, \tag{7}$$

where $G(11';[U])$ means that the propagator is computed in the presence of the external potential. The operator $\hat{S}$ is defined as

$$\begin{aligned}\hat{S} &= \hat{T}\left[\exp\left\{-\text{i}\int_{-\infty}^{\infty}\text{d}t_1\,\hat{\mathcal{U}}_{\text{I}}(t_1)\right\}\right]\\ &= \hat{T}\left[\exp\left\{-\frac{\text{i}}{2}\left[\int_{-\infty}^{\infty}\text{d}(11')\,\hat{\psi}_{\text{I}}(1)U^{\text{hh}}(11')\hat{\psi}_{\text{I}}(1') + \int_{-\infty}^{\infty}\text{d}(11')\,\hat{\psi}_{\text{I}}^{\dagger}(1')U^{\text{ee}}(11')\hat{\psi}_{\text{I}}^{\dagger}(1')\right]\right\}\right].\end{aligned} \tag{8}$$

Here, $\hat{\mathcal{U}}_{\text{I}}(t)$ is the external potential operator defined in Eq. (1) in the interaction picture. In these expressions for the anomalous propagators, the external potential does not appear in the field operators but only in $\hat{S}$.

The first-order variation of $\hat{S}$ as $\hat{\mathcal{U}}$ is varied by an infinitesimal amount $\delta\hat{\mathcal{U}}$ reads

$$\begin{aligned}\delta\hat{S} &= \hat{T}\left[\exp\left(-\text{i}\int_{-\infty}^{\infty}\text{d}t_1\left[\hat{\mathcal{U}}_{\text{I}}(t_1)+\delta\hat{\mathcal{U}}_{\text{I}}(t_1)\right]\right)\right] - \hat{T}\left[\exp\left(-\text{i}\int_{-\infty}^{\infty}\text{d}t_1\,\hat{\mathcal{U}}_{\text{I}}(t_1)\right)\right]\\ &= \hat{T}\left[\hat{S}\left(-\text{i}\int_{-\infty}^{\infty}\text{d}t_1\,\delta\hat{\mathcal{U}}_{\text{I}}(t_1)\right)\right]\\ &= -\frac{\text{i}}{2}\hat{T}\left[\hat{S}\left(\int_{-\infty}^{\infty}\text{d}(11')\,\hat{\psi}_{\text{I}}(1)\delta U^{\text{hh}}(11')\hat{\psi}_{\text{I}}(1') + \int_{-\infty}^{\infty}\text{d}(11')\,\hat{\psi}_{\text{I}}^{\dagger}(1)\delta U^{\text{ee}}(11')\hat{\psi}_{\text{I}}^{\dagger}(1')\right)\right],\end{aligned} \tag{9}$$

where we have defined $\delta U^{\text{hh}}(11') = \delta U^{\text{hh}}(\mathbf{x}_1\mathbf{x}_{1'};t_1)\delta(t_1-t_{1'})$ and $\delta U^{\text{ee}}(11') = \delta U^{\text{ee}}(\mathbf{x}_1\mathbf{x}_{1'};t_1)\delta(t_1-t_{1'})$. The expression of $\delta\hat{S}$ can then be employed to compute the first-order variation of $G^{\text{ee}}$, as follows

$$\begin{aligned}\delta G^{\text{ee}}(1'2';[U]) &= (-\text{i})\frac{\langle\Psi_0|\hat{T}[\delta\hat{S}\hat{\psi}_{\text{I}}^{\dagger}(1')\hat{\psi}_{\text{I}}^{\dagger}(2')]|\Psi_0\rangle}{\langle\Psi_0|\hat{T}[\hat{S}]|\Psi_0\rangle} - G^{\text{ee}}(1'2')\frac{\langle\Psi_0|\hat{T}[\delta\hat{S}]|\Psi_0\rangle}{\langle\Psi_0|\hat{T}[\hat{S}]|\Psi_0\rangle}\\ &= \frac{1}{2}\int\text{d}(12)\,\delta U^{\text{hh}}(12)\left[(-\text{i})^2\frac{\langle\Psi_0|\hat{T}[\hat{S}\hat{\psi}_{\text{I}}(1)\hat{\psi}_{\text{I}}(2)\hat{\psi}_{\text{I}}^{\dagger}(1')\hat{\psi}_{\text{I}}^{\dagger}(2')]|\Psi_0\rangle}{\langle\Psi_0|\hat{T}[\hat{S}]|\Psi_0\rangle} - G^{\text{ee}}(1'2')(-\text{i})\frac{\langle\Psi_0|\hat{T}[\hat{S}\hat{\psi}_{\text{I}}(1)\hat{\psi}_{\text{I}}(2)]|\Psi_0\rangle}{\langle\Psi_0|\hat{T}[\hat{S}]|\Psi_0\rangle}\right]\\ &= \frac{1}{2}\int\text{d}(12)\,\delta U^{\text{hh}}(12)\left[G_2(12;2'1';[U]) - G^{\text{ee}}(1'2';[U])G^{\text{hh}}(12;[U])\right],\end{aligned} \tag{10}$$

where we have set $\delta U^{\text{ee}} = 0$ for the sake of readability but the variation of $G^{\text{ee}}$ with respect to $U^{\text{ee}}$ can easily be obtained by considering $\delta U^{\text{ee}}$ explicitly. Hence, this yields

$$2\frac{\delta G^{\text{ee}}(1'2';[U])}{\delta U^{\text{hh}}(12)} = -G_2(12;1'2';[U]) - G^{\text{ee}}(1'2';[U])G^{\text{hh}}(12;[U]). \tag{11}$$

As readily seen in the previous equation, the derivative of the anomalous Green's function is equal to the sum of two terms. However, because $G^{\text{ee}}(1'2';[U=0]) = 0$, only the first term remains in the absence of the pairing potentials, that is,

$$\left.\frac{\delta G^{\text{ee}}(1'2';[U])}{\delta U^{\text{hh}}(12)}\right|_{U=0} = -\frac{1}{2}G_2(12;1'2'). \tag{12}$$

Note that differentiating $G^{\text{hh}}(12;[U])$ with respect to $U^{\text{ee}}(1'2')$ would yield the same right-hand side. The left-hand side describes the pairing propagator fluctuation and is denoted as [3]

$$K(12;1'2') = \left.\frac{\delta G^{\text{ee}}(1'2';[U])}{\delta U^{\text{hh}}(12)}\right|_{U=0}. \tag{13}$$

## II. EQUATION OF MOTION FOR THE GORKOV PROPAGATOR

In this section, the usual derivation of the Dyson equation through the EOM of $G^{\mathrm{he}}$ (see, for example, the supporting information in Ref. 4 for a detailed derivation) will be extended to the Gorkov propagator $\boldsymbol{G}$ (which has been defined in the main text). As explained in the main text, the aim is to obtain the pp Gorkov-Hedin equations in the presence of an external potential $\hat{\mathcal{U}}(t)$. Hence, the EOM is derived for $\hat{H}'(t) = \hat{H} + \hat{\mathcal{U}}(t)$ accordingly.

### A. EOM for the he component

The time derivative of $G^{\mathrm{he}}$ is

$$\begin{aligned}\mathrm{i}\frac{\partial G^{\mathrm{he}}(11';[U])}{\partial t_1} &= \delta(t_1 - t_{1'})\,\langle\Psi_0|\hat{\psi}(1)\hat{\psi}^\dagger(1') + \hat{\psi}^\dagger(1')\hat{\psi}(1)|\Psi_0\rangle \\ &+ \Theta(t_1 - t_{1'})\,\langle\Psi_0|\Big\{-\mathrm{i}\hat{U}^\dagger_{\hat{H}'}(t_1)\Big[\hat{\psi}(\mathbf{x}_1), \hat{H} + \hat{\mathcal{U}}(t_1)\Big]\hat{U}_{\hat{H}'}(t_1)\Big\}\,\hat{\psi}^\dagger(1')|\Psi_0\rangle \\ &- \Theta(t_{1'} - t_1)\,\langle\Psi_0|\hat{\psi}^\dagger(1')\,\Big\{-\mathrm{i}\hat{U}^\dagger_{\hat{H}'}(t_1)\Big[\hat{\psi}(\mathbf{x}_1), \hat{H} + \hat{\mathcal{U}}(t_1)\Big]\hat{U}_{\hat{H}'}(t_1)\Big\}|\Psi_0\rangle\,.\end{aligned} \tag{14}$$

The first term involves the equal-time anticommutator of an annihilation and a creation operator and therefore becomes $\delta(11')$. The commutator (in the Heisenberg picture) of an annihilation operator with the Hamiltonian and the potential shows up in the two remaining terms. The hh component of $\hat{\mathcal{U}}(t)$ commutes with $\hat{\psi}(\mathbf{x}_1)$. Therefore, only $U^{\mathrm{ee}}$ remains and the EOM becomes

$$\begin{aligned}\mathrm{i}\frac{\partial G^{\mathrm{he}}(11';[U])}{\partial t_1} &= \delta(11') + \int \mathrm{d}3\, h(13)G^{\mathrm{he}}(31';[U]) + \int \mathrm{d}3\, U^{\mathrm{ee}}(31)G^{\mathrm{ee}}(31';[U]) \\ &- \mathrm{i}\int \mathrm{d}(232')\, v(12;32')\lim_{\delta\to 0^+}\,\langle\Psi_0|\hat{T}[\hat{\psi}^\dagger(2^{++})\hat{\psi}(2'^{+})\hat{\psi}(3)\hat{\psi}^\dagger(1')]|\Psi_0\rangle\,.\end{aligned} \tag{15}$$

### B. EOM for the hh component

The time derivative of $G^{\mathrm{hh}}$ is

$$\begin{aligned}\mathrm{i}\frac{\partial G^{\mathrm{hh}}(11';[U])}{\partial t_1} &= \delta(t_1 - t_{1'})\,\langle\Psi_0|\hat{\psi}(1)\hat{\psi}(1') + \hat{\psi}(1')\hat{\psi}(1)|\Psi_0\rangle \\ &+ \Theta(t_1 - t_{1'})\,\langle\Psi_0|\Big\{-\mathrm{i}\hat{U}^\dagger_{\hat{H}'}(t_1)\Big[\hat{\psi}(\mathbf{x}_1), \hat{H} + \hat{\mathcal{U}}(t_1)\Big]\hat{U}_{\hat{H}'}(t_1)\Big\}\,\hat{\psi}(1')|\Psi_0\rangle \\ &- \Theta(t_{1'} - t_1)\,\langle\Psi_0|\hat{\psi}(1')\,\Big\{-\mathrm{i}\hat{U}^\dagger_{\hat{H}'}(t_1)\Big[\hat{\psi}(\mathbf{x}_1), \hat{H} + \hat{\mathcal{U}}(t_1)\Big]\hat{U}_{\hat{H}'}(t_1)\Big\}|\Psi_0\rangle\,.\end{aligned} \tag{16}$$

The first term is equal to the equal-time anticommutator of two annihilation operators and, therefore, is zero while the two remaining terms are dealt with as above, that is,

$$\begin{aligned}\mathrm{i}\frac{\partial G^{\mathrm{hh}}(11';[U])}{\partial t_1} &= \int \mathrm{d}3\, h(13)G^{\mathrm{hh}}(31';[U]) + \int \mathrm{d}3\, U^{\mathrm{ee}}(31)G^{\mathrm{eh}}(31';[U]) \\ &- \mathrm{i}\int \mathrm{d}(232')\, v(12;32')\lim_{\delta\to 0^+}\,\langle\Psi_0|\hat{T}[\hat{\psi}^\dagger(2^{++})\hat{\psi}(2'^{+})\hat{\psi}(3)\hat{\psi}(1')]|\Psi_0\rangle\,.\end{aligned} \tag{17}$$

### C. EOM for the ee component

The time derivative of $G^{\mathrm{ee}}$ is

$$\begin{aligned}\mathrm{i}\frac{\partial G^{\mathrm{ee}}(11';[U])}{\partial t_1} &= \delta(t_1 - t_{1'})\,\langle\Psi_0|\hat{\psi}^\dagger(1)\hat{\psi}^\dagger(1') + \hat{\psi}^\dagger(1')\hat{\psi}^\dagger(1)|\Psi_0\rangle \\ &+ \Theta(t_1 - t_{1'})\,\langle\Psi_0|\Big\{-\mathrm{i}\hat{U}^\dagger_{\hat{H}'}(t_1)\Big[\hat{\psi}^\dagger(\mathbf{x}_1), \hat{H} + \hat{\mathcal{U}}(t_1)\Big]\hat{U}_{\hat{H}'}(t_1)\Big\}\,\hat{\psi}^\dagger(1')|\Psi_0\rangle \\ &- \Theta(t_{1'} - t_1)\,\langle\Psi_0|\hat{\psi}^\dagger(1')\,\Big\{-\mathrm{i}\hat{U}^\dagger_{\hat{H}'}(t_1)\Big[\hat{\psi}^\dagger(\mathbf{x}_1), \hat{H} + \hat{\mathcal{U}}(t_1)\Big]\hat{U}_{\hat{H}'}(t_1)\Big\}|\Psi_0\rangle\,.\end{aligned} \tag{18}$$

The first term is equal to the equal-time anticommutator of two creation operators and, therefore, is zero. In this case, only $U^{\text{hh}}$ remains in the Hamiltonian commutator because the ee component of $\hat{\mathcal{U}}(t)$ commutes with $\hat{\psi}^\dagger(\mathbf{x}_1)$ and the EOM reads

$$\mathrm{i}\frac{\partial G^{\text{ee}}(11';[U])}{\partial t_1} = -\int \mathrm{d}3\, h(31) G^{\text{ee}}(31';[U]) + \int \mathrm{d}3\, U^{\text{hh}}(31) G^{\text{he}}(31';[U]) + \mathrm{i}\int \mathrm{d}(232')\, v(32;12') \lim_{\delta\to 0^+} \langle \Psi_0|\hat{T}[\hat{\psi}^\dagger(3)\hat{\psi}^\dagger(2^-)\hat{\psi}(2'^{--})\hat{\psi}^\dagger(1')]|\Psi_0\rangle \,. \quad (19)$$

### D. EOM for the eh component

The time derivative of $G^{\text{eh}}$ is

$$\begin{aligned}\mathrm{i}\frac{\partial G^{\text{eh}}(11';[U])}{\partial t_1} &= \delta(t_1 - t_{1'}) \langle \Psi_0|\hat{\psi}^\dagger(1)\hat{\psi}(1') + \hat{\psi}(1')\hat{\psi}^\dagger(1)|\Psi_0\rangle \\ &+ \Theta(t_1 - t_{1'}) \langle \Psi_0|\left(-\mathrm{i}\hat{U}^\dagger_{\hat{H}'}(t_1)\left[\hat{\psi}^\dagger(\mathbf{x}_1), \hat{H} + \hat{\mathcal{U}}(t_1)\right]\hat{U}_{\hat{H}'}(t_1)\right)\hat{\psi}(1')|\Psi_0\rangle \\ &- \Theta(t_{1'} - t_1) \langle \Psi_0|\hat{\psi}(1')\left(-\mathrm{i}\hat{U}^\dagger_{\hat{H}'}(t_1)\left[\hat{\psi}^\dagger(\mathbf{x}_1), \hat{H} + \hat{\mathcal{U}}(t_1)\right]\hat{U}_{\hat{H}'}(t_1)\right)|\Psi_0\rangle \,.\end{aligned} \quad (20)$$

Therefore, the final EOM is

$$\mathrm{i}\frac{\partial G^{\text{eh}}(11';[U])}{\partial t_1} = \delta(11') - \int \mathrm{d}3\, h(31) G^{\text{eh}}(31';[U]) + \int \mathrm{d}3\, U^{\text{hh}}(31) G^{\text{hh}}(31';[U]) + \mathrm{i}\int \mathrm{d}(232')\, v(32;12') \lim_{\delta\to 0^+} \langle \Psi_0|\hat{T}[\hat{\psi}^\dagger(3)\hat{\psi}^\dagger(2^-)\hat{\psi}(2'^{--})\hat{\psi}(1')]|\Psi_0\rangle \,. \quad (21)$$

### E. Gathering components

The four previous equations can be gathered to obtain the EOM for the Gorkov propagator

$$\mathrm{i}\frac{\partial \boldsymbol{G}(11';[U])}{\partial t_1} = \begin{pmatrix}\delta(11') & 0\\ 0 & \delta(11')\end{pmatrix} + \int \mathrm{d}3 \begin{pmatrix} h(13) & 0 \\ 0 & -h(31)\end{pmatrix} \boldsymbol{G}(31';[U]) + \int \mathrm{d}3 \begin{pmatrix} 0 & U^{\text{ee}}(31) \\ U^{\text{hh}}(31) & 0\end{pmatrix} \boldsymbol{G}(31';[U]) + \mathrm{i}\int \mathrm{d}(232') \lim_{\delta\to 0^+} \begin{pmatrix} v(12^{--};32'^-) & 0 \\ 0 & -v(32^+;12'^{++})\end{pmatrix} \boldsymbol{G}_2(2'3;21';[U]), \quad (22)$$

where $\boldsymbol{G}_2$ stands for the following generalization of the two-body Green's function

$$\boldsymbol{G}_2(12;1'2';[U]) = (-\mathrm{i})^2 \langle \Psi_0|\hat{T}\left[\begin{pmatrix}\hat{\psi}(1)\hat{\psi}(2)\hat{\psi}^\dagger(2')\hat{\psi}^\dagger(1') & \hat{\psi}(1)\hat{\psi}(2)\hat{\psi}(2')\hat{\psi}^\dagger(1') \\ \hat{\psi}(1)\hat{\psi}^\dagger(2)\hat{\psi}^\dagger(2')\hat{\psi}^\dagger(1') & \hat{\psi}(1)\hat{\psi}^\dagger(2)\hat{\psi}(2')\hat{\psi}^\dagger(1')\end{pmatrix}\right]|\Psi_0\rangle \,. \quad (23)$$

The independent-particle Gorkov propagator is defined as

$$\int \mathrm{d}3 \begin{pmatrix}\delta(13)\frac{\partial}{\partial t_3} - h(13) & 0 \\ 0 & \delta(13)\frac{\partial}{\partial t_3} + h(31)\end{pmatrix} \boldsymbol{G}_0(31') = \begin{pmatrix}\delta(11') & 0 \\ 0 & \delta(11')\end{pmatrix}, \quad (24)$$

or, equivalently,

$$\boldsymbol{G}_0^{-1}(13) = \begin{pmatrix}\delta(13)\frac{\partial}{\partial t_3} - h(13) & 0 \\ 0 & \delta(13)\frac{\partial}{\partial t_3} + h(31)\end{pmatrix}. \quad (25)$$

Therefore, the matrix form of the Dyson equation is finally obtained as

$$\boldsymbol{G}(11') = \boldsymbol{G}_0(11') + \int \mathrm{d}(22')\, \boldsymbol{G}_0(12)\left[\boldsymbol{\Sigma}(22') + \boldsymbol{U}(22')\right]\boldsymbol{G}(2'1'), \quad (26)$$

where the self-energy is

$$\boldsymbol{\Sigma}(11') = -\mathrm{i}\int \mathrm{d}(232'3') \begin{pmatrix} v(12^{--};32'^{-}) & 0 \\ 0 & -v(32^{+};12'^{++}) \end{pmatrix} \boldsymbol{G}_2(2'3;23')\boldsymbol{G}^{-1}(3'1'), \tag{27}$$

and the potential is

$$\boldsymbol{U}(11') = \begin{pmatrix} 0 & U^{\mathrm{ee}}(11') \\ U^{\mathrm{hh}}(11') & 0 \end{pmatrix}. \tag{28}$$

Note that $U^{\mathrm{ee}}$ appears in the hh component of Nambu's matrix formalism and vice-versa. In the above equations, and from hereon, the explicit $U$-dependence and the $\lim_{\delta\to 0^+}$ symbol has been removed for the sake of conciseness.

## III. CLOSED SET OF EQUATIONS WITHOUT EFFECTIVE INTERACTIONS

Now that the EOM for the Gorkov propagator has been obtained in Sec. II, the next step is to get rid of $\boldsymbol{G}_2$ to obtain a closed set of equations for $\boldsymbol{G}$. To do so, the Schwinger relation [see Eq. (11)] also needs to be generalized to the Gorkov propagator. A straightforward extension of the derivation presented in Sec. I leads to

$$\boldsymbol{G}_2(12;1'2') = \begin{pmatrix} -2\dfrac{\delta G^{\mathrm{ee}}(1'2')}{\delta U^{\mathrm{hh}}(12)} - G^{\mathrm{ee}}(1'2')G^{\mathrm{hh}}(12) & -2\dfrac{\delta G^{\mathrm{eh}}(1'2')}{\delta U^{\mathrm{hh}}(12)} - G^{\mathrm{eh}}(1'2')G^{\mathrm{hh}}(12) \\ -2\dfrac{\delta G^{\mathrm{he}}(12')}{\delta U^{\mathrm{ee}}(21')} - G^{\mathrm{he}}(12')G^{\mathrm{ee}}(21') & -2\dfrac{\delta G^{\mathrm{hh}}(12')}{\delta U^{\mathrm{ee}}(21')} - G^{\mathrm{hh}}(12')G^{\mathrm{ee}}(21') \end{pmatrix}. \tag{29}$$

Note that the usual Schwinger relation in terms of a number-conserving external potential can also be generalized to $\boldsymbol{G}$ and can be used, for example, to derive $GW$-like approximations for the anomalous self-energies (see Ref. [5] for more details).

We start by focusing on the self-energy coming from the second term in the generalized Schwinger relation

$$\mathrm{i}\int \mathrm{d}(232'3') \begin{pmatrix} v(12^{--};32'^{-}) & 0 \\ 0 & -v(32^{+};12'^{++}) \end{pmatrix} \begin{pmatrix} G^{\mathrm{ee}}(23')G^{\mathrm{hh}}(2'3) & G^{\mathrm{eh}}(23')G^{\mathrm{hh}}(2'3) \\ G^{\mathrm{he}}(2'3')G^{\mathrm{ee}}(32) & G^{\mathrm{hh}}(2'3')G^{\mathrm{ee}}(32) \end{pmatrix} \boldsymbol{G}^{-1}(3'1'). \tag{30}$$

The matrix of products of Green's functions can be factorized if the dummy indices 2 and $2'$ are swapped in the second row

$$\begin{pmatrix} G^{\mathrm{ee}}(23')G^{\mathrm{hh}}(2'3) & G^{\mathrm{eh}}(23')G^{\mathrm{hh}}(2'3) \\ G^{\mathrm{he}}(23')G^{\mathrm{ee}}(32') & G^{\mathrm{hh}}(23')G^{\mathrm{ee}}(32') \end{pmatrix} = \begin{pmatrix} 0 & G^{\mathrm{hh}}(2'3) \\ G^{\mathrm{ee}}(32') & 0 \end{pmatrix} \begin{pmatrix} G^{\mathrm{he}}(23') & G^{\mathrm{hh}}(23') \\ G^{\mathrm{ee}}(23') & G^{\mathrm{eh}}(23') \end{pmatrix}. \tag{31}$$

This factorization is particularly convenient because it allows a simplification with the inverse Gorkov propagator in the self-energy

$$\mathrm{i}\int \mathrm{d}(232') \begin{pmatrix} v(12^{--};32'^{-}) & 0 \\ 0 & -v(32'^{+};12^{++}) \end{pmatrix} \begin{pmatrix} 0 & G^{\mathrm{hh}}(2'3) \\ G^{\mathrm{ee}}(32') & 0 \end{pmatrix} \delta(21'), \tag{32}$$

which finally gives

$$\boldsymbol{\Sigma}_{\mathrm{B}}(11') = \mathrm{i}\int \mathrm{d}(2'3) \begin{pmatrix} 0 & v(11'^{--};32'^{-})G^{\mathrm{hh}}(2'3) \\ -v(32'^{+};11'^{++})G^{\mathrm{ee}}(32') & 0 \end{pmatrix}. \tag{33}$$

Here, we recognize the first-order anomalous self-energies which appear, for example, in Hartree-Fock-Bogoliubov theory [6]. This static term will be referred to as the Bogoliubov (B) self-energy $\boldsymbol{\Sigma}_{\mathrm{B}}$ in the following. The remaining self-energy contains the Hartree, exchange, and correlation diagrams and will be denoted as $\boldsymbol{\Sigma}_{\mathrm{Hxc}}$. The total self-energy is thus

$$\boldsymbol{\Sigma}(11') = \boldsymbol{\Sigma}_{\mathrm{B}}(11') + \boldsymbol{\Sigma}_{\mathrm{Hxc}}(11'). \tag{34}$$

The remaining term in Eq. (29) is denoted as

$$-2\begin{pmatrix} \dfrac{\delta G^{\mathrm{ee}}(23')}{\delta U^{\mathrm{hh}}(2'3)} & \dfrac{\delta G^{\mathrm{eh}}(23')}{\delta U^{\mathrm{hh}}(2'3)} \\ \dfrac{\delta G^{\mathrm{he}}(23')}{\delta U^{\mathrm{ee}}(32')} & \dfrac{\delta G^{\mathrm{hh}}(23')}{\delta U^{\mathrm{ee}}(32')} \end{pmatrix} = -2\begin{pmatrix} 0 & \dfrac{\delta}{\delta U^{\mathrm{hh}}(2'3)} \\ \dfrac{\delta}{\delta U^{\mathrm{ee}}(32')} & 0 \end{pmatrix} [\boldsymbol{G}(23')], \tag{35}$$

where the dummy indices of the second row have been swapped again. This term is dealt with as usual, *i.e.* by transforming it to the derivative of the inverse propagator. Such a relation is obtained by differentiating

$$\int \mathrm{d}3'\, \boldsymbol{G}(23')\boldsymbol{G}^{-1}(3'1') = \boldsymbol{\delta}(21'), \tag{36}$$

where

$$\boldsymbol{\delta}(11') = \begin{pmatrix} \delta(11') & 0 \\ 0 & \delta(11') \end{pmatrix} \tag{37}$$

is Nambu's generalization of the Dirac delta function. The resulting relation is

$$\begin{pmatrix} 0 & \dfrac{\delta}{\delta U^{\mathrm{hh}}(2'3)} \\ \dfrac{\delta}{\delta U^{\mathrm{ee}}(32')} & 0 \end{pmatrix} [\boldsymbol{G}(23')]\boldsymbol{G}^{-1}(3'1') = -\begin{pmatrix} G^{\mathrm{ee}}(23') & G^{\mathrm{eh}}(23') \\ 0 & 0 \end{pmatrix} \begin{pmatrix} \dfrac{\delta(G^{-1})^{\mathrm{he}}(3'1')}{\delta U^{\mathrm{hh}}(2'3)} & \dfrac{\delta(G^{-1})^{\mathrm{hh}}(3'1')}{\delta U^{\mathrm{hh}}(2'3)} \\ \dfrac{\delta(G^{-1})^{\mathrm{ee}}(3'1')}{\delta U^{\mathrm{hh}}(2'3)} & \dfrac{\delta(G^{-1})^{\mathrm{eh}}(3'1')}{\delta U^{\mathrm{hh}}(2'3)} \end{pmatrix} \tag{38}$$

$$-\begin{pmatrix} 0 & 0 \\ G^{\mathrm{he}}(23') & G^{\mathrm{hh}}(23') \end{pmatrix} \begin{pmatrix} \dfrac{\delta(G^{-1})^{\mathrm{he}}(3'1')}{\delta U^{\mathrm{ee}}(32')} & \dfrac{\delta(G^{-1})^{\mathrm{hh}}(3'1')}{\delta U^{\mathrm{ee}}(32')} \\ \dfrac{\delta(G^{-1})^{\mathrm{ee}}(3'1')}{\delta U^{\mathrm{ee}}(32')} & \dfrac{\delta(G^{-1})^{\mathrm{eh}}(3'1')}{\delta U^{\mathrm{ee}}(32')} \end{pmatrix}, \tag{39}$$

and the corresponding self-energy reads

$$\begin{aligned} \boldsymbol{\Sigma}_{\mathrm{Hxc}}(11') = 2\mathrm{i} \int \mathrm{d}(232'3') &\begin{pmatrix} v(12^{--};32'^{-}) & 0 \\ 0 & -v(32'^{+};12^{++}) \end{pmatrix} \\ &\times \left[ \begin{pmatrix} G^{\mathrm{ee}}(23') & G^{\mathrm{eh}}(23') \\ 0 & 0 \end{pmatrix} \boldsymbol{\Gamma}^{\mathrm{hh}}(2'3;3'1') + \begin{pmatrix} 0 & 0 \\ G^{\mathrm{he}}(23') & G^{\mathrm{hh}}(23') \end{pmatrix} \boldsymbol{\Gamma}^{\mathrm{ee}}(32';3'1') \right], \end{aligned} \tag{40}$$

where the vertex functions have been defined as

$$\boldsymbol{\Gamma}^{\mathrm{hh}}(2'3;3'1') = -\frac{\delta \boldsymbol{G}^{-1}(3'1')}{\delta U^{\mathrm{hh}}(2'3)}, \qquad \boldsymbol{\Gamma}^{\mathrm{ee}}(32';3'1') = -\frac{\delta \boldsymbol{G}^{-1}(3'1')}{\delta U^{\mathrm{ee}}(32')}. \tag{41}$$

From hereon, integration over repeated indices is assumed in the expression of the self-energy.

Before introducing effective interactions through chain rules, the lowest-order self-energy approximation coming from Eq. (40) is investigated. It is obtained using the simplest approximations of $\boldsymbol{\Gamma}_0^{\mathrm{hh}}$ and $\boldsymbol{\Gamma}_0^{\mathrm{ee}}$, that is,

$$\boldsymbol{\Gamma}_0^{\mathrm{hh}}(2'3;3'1') = \frac{1}{2}\begin{pmatrix} 0 & 0 \\ \delta(3'2')\delta(1'3) - \delta(3'3)\delta(1'2') & 0 \end{pmatrix}, \quad \boldsymbol{\Gamma}_0^{\mathrm{ee}}(32';3'1') = \frac{1}{2}\begin{pmatrix} 0 & \delta(3'3)\delta(1'2') - \delta(3'2')\delta(1'3) \\ 0 & 0 \end{pmatrix}, \tag{42}$$

where we relied on the following identity

$$\frac{\delta U^{\mathrm{hh}}(12)}{\delta U^{\mathrm{hh}}(34)} = \frac{1}{2}\left[\delta(13)\delta(24) - \delta(14)\delta(23)\right]. \tag{43}$$

The usual functional derivative $\delta U^{\mathrm{hh}}(12)/\delta U^{\mathrm{hh}}(34) = \delta(13)\delta(24)$ is also mathematically correct. However, it does break the antisymmetry of the equations. Therefore, one must rely on constrained functional derivatives that preserve the antisymmetric nature of the problem. We refer the interested reader to Ref. [7] for details on this subtle mathematical point. These approximations lead to a diagonal self-energy

$$\begin{aligned} \boldsymbol{\Sigma}_{\mathrm{Hx}}(11') = -\mathrm{i} \int \mathrm{d}(22') &\begin{pmatrix} v(12^{--};1'2'^{-})G^{\mathrm{he}}(2'2) & 0 \\ 0 & v(1'2'^{+};12^{++})G^{\mathrm{he}}(22') \end{pmatrix} \\ &+ \mathrm{i} \int \mathrm{d}(232') \begin{pmatrix} v(12^{--};2'1'^{-})G^{\mathrm{he}}(2'2) & 0 \\ 0 & v(2'1'^{+};12^{++})G^{\mathrm{he}}(22') \end{pmatrix}, \end{aligned} \tag{44}$$

where the diagonal terms are recognized to be the Hartree-exchange first-order self-energy. Hence, once combined with the self-energy defined in Eq. (33), the self-energy $\boldsymbol{\Sigma}$ corresponding to the lowest-order vertex approximation is equivalent to the Hartree-Fock-Bogoliubov approximation.

## IV. PARTICLE-PARTICLE GORKOV-HEDIN EQUATIONS

The self-energy will now be expressed in terms of effective interactions in order to obtain an analog of Hedin's equations. Mathematically, this is done starting from Eq. (40) and using the chain rule with respect to the two anomalous total potential $V^{\rm ee} = \Sigma_{\rm B}^{\rm ee} + U^{\rm hh}$ and $V^{\rm hh} = \Sigma_{\rm B}^{\rm hh} + U^{\rm ee}$. Following this procedure, one gets

$$\begin{aligned}\boldsymbol{\Sigma}_{\rm Hxc}(11') = 2{\rm i}\Bigg[&v(12;32')\begin{pmatrix} G^{\rm ee}(2^{++}3') & G^{\rm eh}(2^{++}3') \\ 0 & 0\end{pmatrix}\left\{\frac{\delta V^{\rm ee}(44')}{\delta U^{\rm hh}(2'^{+}3)}\tilde{\boldsymbol{\Gamma}}^{\rm ee}(44';3'1') + \frac{\delta V^{\rm hh}(44')}{\delta U^{\rm hh}(2'^{+}3)}\tilde{\boldsymbol{\Gamma}}^{\rm hh}(44';3'1')\right\} \\ &-v(32';12)\begin{pmatrix} 0 & 0 \\ G^{\rm he}(2^{--}3') & G^{\rm hh}(2^{--}3')\end{pmatrix}\left\{\frac{\delta V^{\rm ee}(44')}{\delta U^{\rm ee}(32'^{-})}\tilde{\boldsymbol{\Gamma}}^{\rm ee}(44';3'1') + \frac{\delta V^{\rm hh}(44')}{\delta U^{\rm ee}(32'^{-})}\tilde{\boldsymbol{\Gamma}}^{\rm hh}(44';3'1')\right\}\Bigg], \quad (45)\end{aligned}$$

where the irreducible vertex functions have been defined as

$$\tilde{\boldsymbol{\Gamma}}^{\rm hh}(44';3'1') = -\frac{\delta \boldsymbol{G}^{-1}(3'1')}{\delta V^{\rm hh}(44')}, \qquad \tilde{\boldsymbol{\Gamma}}^{\rm ee}(44';3'1') = -\frac{\delta \boldsymbol{G}^{-1}(3'1')}{\delta V^{\rm ee}(44')}. \quad (46)$$

The quantities $\delta V/\delta U$ are the analogs of the inverse dielectric matrix in traditional Hedin's equations. As readily seen from Eq. (45), there are four such terms. This suggests to introduce a generalized effective interaction in Nambu's formalism, such that

$$\boldsymbol{T}(12;44') = \begin{pmatrix} T^{\rm he}(12;44') & T^{\rm hh}(12;44') \\ T^{\rm ee}(12;44') & T^{\rm eh}(12;44')\end{pmatrix} = 2\begin{pmatrix} v(12;32') & 0 \\ 0 & -v(32';12)\end{pmatrix}\begin{pmatrix} \dfrac{\delta V^{\rm ee}(44')}{\delta U^{\rm hh}(2'^{+}3)} & \dfrac{\delta V^{\rm hh}(44')}{\delta U^{\rm hh}(2'^{+}3)} \\ \dfrac{\delta V^{\rm ee}(44')}{\delta U^{\rm ee}(32'^{-})} & \dfrac{\delta V^{\rm hh}(44')}{\delta U^{\rm ee}(32'^{-})}\end{pmatrix}. \quad (47)$$

Using these notations, the self-energy (45) becomes

$$\begin{aligned}\boldsymbol{\Sigma}_{\rm Hxc}(11') = {\rm i}\Bigg[&\begin{pmatrix} G^{\rm ee}(2^{++}3') & G^{\rm eh}(2^{++}3') \\ 0 & 0\end{pmatrix}\left\{T^{\rm he}(12;44')\tilde{\boldsymbol{\Gamma}}^{\rm ee}(44';3'1') + T^{\rm hh}(12;44')\tilde{\boldsymbol{\Gamma}}^{\rm hh}(44';3'1')\right\} \\ &+\begin{pmatrix} 0 & 0 \\ G^{\rm he}(2^{--}3') & G^{\rm hh}(2^{--}3')\end{pmatrix}\left\{T^{\rm ee}(12;44')\tilde{\boldsymbol{\Gamma}}^{\rm ee}(44';3'1') + T^{\rm eh}(12;44')\tilde{\boldsymbol{\Gamma}}^{\rm hh}(44';3'1')\right\}\Bigg], \quad (48)\end{aligned}$$

or, equivalently,

$$\begin{aligned}\boldsymbol{\Sigma}_{\rm Hxc}(11') = {\rm i}\Bigg[&\begin{pmatrix} T^{\rm he}(12;44') & 0 \\ 0 & T^{\rm ee}(12;44')\end{pmatrix}\begin{pmatrix} G^{\rm ee}(2^{++}3') & G^{\rm eh}(2^{++}3') \\ G^{\rm he}(2^{--}3') & G^{\rm hh}(2^{--}3')\end{pmatrix}\tilde{\boldsymbol{\Gamma}}^{\rm ee}(44';3'1') \\ &+\begin{pmatrix} T^{\rm hh}(12;44') & 0 \\ 0 & T^{\rm eh}(12;44')\end{pmatrix}\begin{pmatrix} G^{\rm ee}(2^{++}3') & G^{\rm eh}(2^{++}3') \\ G^{\rm he}(2^{--}3') & G^{\rm hh}(2^{--}3')\end{pmatrix}\tilde{\boldsymbol{\Gamma}}^{\rm hh}(44';3'1')\Bigg]. \quad (49)\end{aligned}$$

The next step is to study the effective interaction $\boldsymbol{T}$ defined in Eq. (47). In particular, our aim is to express it as a Dyson equation and then investigate the effect of the inner-vertex corrections. The derivatives of the total potentials yield two terms

$$\boldsymbol{T}(12;44') = 2\begin{pmatrix} v(12;32') & 0 \\ 0 & -v(32';12)\end{pmatrix}\left[\begin{pmatrix} \dfrac{\delta U^{\rm hh}(44')}{\delta U^{\rm hh}(2'^{+}3)} & \dfrac{\delta U^{\rm ee}(44')}{\delta U^{\rm hh}(2'^{+}3)} \\ \dfrac{\delta U^{\rm hh}(44')}{\delta U^{\rm ee}(32'^{-})} & \dfrac{\delta U^{\rm ee}(44')}{\delta U^{\rm ee}(32'^{-})}\end{pmatrix} + \begin{pmatrix} \dfrac{\delta \Sigma_{\rm B}^{\rm ee}(44')}{\delta U^{\rm hh}(2'^{+}3)} & \dfrac{\delta \Sigma_{\rm B}^{\rm hh}(44')}{\delta U^{\rm hh}(2'^{+}3)} \\ \dfrac{\delta \Sigma_{\rm B}^{\rm ee}(44')}{\delta U^{\rm ee}(32'^{-})} & \dfrac{\delta \Sigma_{\rm B}^{\rm hh}(44')}{\delta U^{\rm ee}(32'^{-})}\end{pmatrix}\right], \quad (50)$$

which can be recast as

$$\begin{aligned}\boldsymbol{T}(12;44') = 2\begin{pmatrix} v(12;32') & 0 \\ 0 & -v(32';12)\end{pmatrix}\Bigg[&\begin{pmatrix} \dfrac{\delta U^{\rm hh}(44')}{\delta U^{\rm hh}(2'^{+}3)} & 0 \\ 0 & \dfrac{\delta U^{\rm ee}(44')}{\delta U^{\rm ee}(32'^{-})}\end{pmatrix} \\ &+{\rm i}\begin{pmatrix} \dfrac{\delta G^{\rm ee}(5'5)}{\delta U^{\rm hh}(2'^{+}3)} & \dfrac{\delta G^{\rm hh}(5'5)}{\delta U^{\rm hh}(2'^{+}3)} \\ \dfrac{\delta G^{\rm ee}(5'5)}{\delta U^{\rm ee}(32'^{-})} & \dfrac{\delta G^{\rm hh}(5'5)}{\delta U^{\rm ee}(32'^{-})}\end{pmatrix}\begin{pmatrix} -v(5'5^{+};44'^{++}) & 0 \\ 0 & -v(44'^{--};5'5^{-})\end{pmatrix}\Bigg]. \quad (51)\end{aligned}$$

To obtain the desired Dyson equation, the next step consists of applying the chain rule on each derivative and factorizing it as a matrix product, which yields

$$\boldsymbol{T}(12;44') = \begin{pmatrix} v(12;4'4) & 0 \\ 0 & -v(44';12) \end{pmatrix} - \begin{pmatrix} v(12;44') & 0 \\ 0 & -v(4'4;12) \end{pmatrix}$$
$$-2\mathrm{i}\begin{pmatrix} v(12;32') & 0 \\ 0 & -v(32';12) \end{pmatrix} \begin{pmatrix} \frac{\delta V^{\mathrm{ee}}(66')}{\delta U^{\mathrm{hh}}(2'^{+}3)} & \frac{\delta V^{\mathrm{hh}}(66')}{\delta U^{\mathrm{hh}}(2'^{+}3)} \\ \frac{\delta V^{\mathrm{ee}}(66')}{\delta U^{\mathrm{ee}}(2'^{-}3)} & \frac{\delta V^{\mathrm{hh}}(66')}{\delta U^{\mathrm{ee}}(2'^{-}3)} \end{pmatrix} \begin{pmatrix} \frac{\delta G^{\mathrm{ee}}(5'5)}{\delta V^{\mathrm{ee}}(66')} & \frac{\delta G^{\mathrm{hh}}(5'5)}{\delta V^{\mathrm{ee}}(66')} \\ \frac{\delta G^{\mathrm{ee}}(5'5)}{\delta V^{\mathrm{hh}}(66')} & \frac{\delta G^{\mathrm{hh}}(5'5)}{\delta V^{\mathrm{hh}}(66')} \end{pmatrix} \begin{pmatrix} v(5'5^{+};44'^{++}) & 0 \\ 0 & v(44'^{--};5'5^{-}) \end{pmatrix}. \tag{52}$$

One can then clearly recognize the generalized $T$-matrix

$$\boldsymbol{T}(12;44') = \begin{pmatrix} v(12;4'4) & 0 \\ 0 & v(4'4;12) \end{pmatrix} - \begin{pmatrix} v(12;44') & 0 \\ 0 & v(44';12) \end{pmatrix}$$
$$- \mathrm{i}\boldsymbol{T}(12;66') \begin{pmatrix} \frac{\delta G^{\mathrm{ee}}(5'5)}{\delta V^{\mathrm{ee}}(66')} & \frac{\delta G^{\mathrm{hh}}(5'5)}{\delta V^{\mathrm{ee}}(66')} \\ \frac{\delta G^{\mathrm{ee}}(5'5)}{\delta V^{\mathrm{hh}}(66')} & \frac{\delta G^{\mathrm{hh}}(5'5)}{\delta V^{\mathrm{hh}}(66')} \end{pmatrix} \begin{pmatrix} v(5'5^{+};44'^{++}) & 0 \\ 0 & v(44'^{--};5'5^{-}) \end{pmatrix}. \tag{53}$$

The previous equation can be written in the more familiar form

$$\boldsymbol{T}(12;44') = -\bar{\boldsymbol{V}}(12;44') - \boldsymbol{T}(12;66')\tilde{\boldsymbol{K}}(66';5'5)\boldsymbol{V}(5'5^{+};44'^{++}), \tag{54}$$

by introducing the matrix form of the Coulomb potential

$$\boldsymbol{V}(12^{+};1'2'^{++}) = \begin{pmatrix} v(12^{+};1'2'^{++}) & 0 \\ 0 & v(1'2'^{--};12^{-}) \end{pmatrix}, \tag{55}$$

and its antisymmetric counterpart $\bar{\boldsymbol{V}}(12;1'2') = \boldsymbol{V}(12;1'2') - \boldsymbol{V}(12;2'1')$. The kernel $\tilde{\boldsymbol{K}}$ of the Dyson equation is equal to

$$\tilde{\boldsymbol{K}}(66';5'5) = \mathrm{i}\begin{pmatrix} \frac{\delta G^{\mathrm{ee}}(5'5)}{\delta V^{\mathrm{ee}}(66')} & \frac{\delta G^{\mathrm{hh}}(5'5)}{\delta V^{\mathrm{ee}}(66')} \\ \frac{\delta G^{\mathrm{ee}}(5'5)}{\delta V^{\mathrm{hh}}(66')} & \frac{\delta G^{\mathrm{hh}}(5'5)}{\delta V^{\mathrm{hh}}(66')} \end{pmatrix} = \mathrm{i}\begin{pmatrix} [\boldsymbol{G}(5'7)\tilde{\boldsymbol{\Gamma}}^{\mathrm{ee}}(66';77')\boldsymbol{G}(7'5)]^{\mathrm{ee}} & [\boldsymbol{G}(5'7)\tilde{\boldsymbol{\Gamma}}^{\mathrm{ee}}(66';77')\boldsymbol{G}(7'5)]^{\mathrm{hh}} \\ [\boldsymbol{G}(5'7)\tilde{\boldsymbol{\Gamma}}^{\mathrm{hh}}(66';77')\boldsymbol{G}(7'5)]^{\mathrm{ee}} & [\boldsymbol{G}(5'7)\tilde{\boldsymbol{\Gamma}}^{\mathrm{hh}}(66';77')\boldsymbol{G}(7'5)]^{\mathrm{hh}} \end{pmatrix}, \tag{56}$$

where $[\boldsymbol{G}\tilde{\boldsymbol{\Gamma}}^{\mathrm{ee}}\boldsymbol{G}]^{\mathrm{ee}}$ stands for the ee block of the product matrix.

The stage is now set to study the self-energy and effective interaction coming from the lowest-order approximation of the irreducible vertex functions

$$\tilde{\boldsymbol{\Gamma}}_0^{\mathrm{hh}}(44';3'1') = \frac{1}{2}\begin{pmatrix} 0 & \delta(3'4)\delta(1'4') - \delta(3'4')\delta(1'4) \\ 0 & 0 \end{pmatrix}, \quad \tilde{\boldsymbol{\Gamma}}_0^{\mathrm{ee}}(44';3'1') = \frac{1}{2}\begin{pmatrix} 0 & 0 \\ \delta(3'4)\delta(1'4') - \delta(3'4')\delta(1'4) & 0 \end{pmatrix}. \tag{57}$$

The corresponding self-energy approximation is

$$\boldsymbol{\Sigma}_{\mathrm{Hxc}}(11') = \mathrm{i}\begin{pmatrix} G^{\mathrm{eh}}(2^{++}3')T^{\mathrm{he}}(12;3'1') & G^{\mathrm{ee}}(2^{++}3')T^{\mathrm{hh}}(12;3'1') \\ G^{\mathrm{hh}}(2^{--}3')T^{\mathrm{ee}}(12;3'1') & G^{\mathrm{he}}(2^{--}3')T^{\mathrm{eh}}(12;3'1') \end{pmatrix}. \tag{58}$$

To obtain the effective interaction $T$ corresponding to the lowest-order inner-vertex correction, one first needs to

compute

$$
\begin{aligned}
\boldsymbol{G}(5'7)\tilde{\boldsymbol{\Gamma}}_0^{\text{ee}}(66';77')\boldsymbol{G}(7'5) &= \frac{1}{2}\boldsymbol{G}(5'7)\begin{pmatrix} 0 & 0 \\ \delta(67)\delta(6'7')-\delta(67')\delta(6'7) & 0\end{pmatrix}\boldsymbol{G}(7'5) \\
&= \frac{1}{2}[\delta(67)\delta(6'7')-\delta(67')\delta(6'7)]\boldsymbol{G}(5'7)\begin{pmatrix} 0 & 0 \\ G^{\text{he}}(7'5) & G^{\text{hh}}(7'5)\end{pmatrix} \\
&= \frac{1}{2}[\delta(67)\delta(6'7')-\delta(67')\delta(6'7)]\begin{pmatrix} G^{\text{hh}}(5'7)G^{\text{he}}(7'5) & G^{\text{hh}}(5'7)G^{\text{hh}}(7'5) \\ G^{\text{eh}}(5'7)G^{\text{he}}(7'5) & G^{\text{eh}}(5'7)G^{\text{hh}}(7'5)\end{pmatrix},
\end{aligned} \tag{59a}
$$

$$
\begin{aligned}
\boldsymbol{G}(5'7)\tilde{\boldsymbol{\Gamma}}_0^{\text{hh}}(66';77')\boldsymbol{G}(7'5) &= \frac{1}{2}\boldsymbol{G}(5'7)\begin{pmatrix} 0 & \delta(67)\delta(6'7')-\delta(67')\delta(6'7) \\ 0 & 0\end{pmatrix}\boldsymbol{G}(7'5) \\
&= \frac{1}{2}[\delta(67)\delta(6'7')-\delta(67')\delta(6'7)]\boldsymbol{G}(5'7)\begin{pmatrix} G^{\text{ee}}(7'5) & G^{\text{eh}}(7'5) \\ 0 & 0\end{pmatrix} \\
&= \frac{1}{2}[\delta(67)\delta(6'7')-\delta(67')\delta(6'7)]\begin{pmatrix} G^{\text{he}}(5'7)G^{\text{ee}}(7'5) & G^{\text{he}}(5'7)G^{\text{eh}}(7'5) \\ G^{\text{ee}}(5'7)G^{\text{ee}}(7'5) & G^{\text{ee}}(5'7)G^{\text{eh}}(7'5)\end{pmatrix}.
\end{aligned} \tag{59b}
$$

Finally, $\tilde{\boldsymbol{K}}$ becomes

$$
\tilde{\boldsymbol{K}}_0(66';5'5) = \frac{\mathrm{i}}{2}[\delta(67)\delta(6'7')-\delta(67')\delta(6'7)]\begin{pmatrix} G^{\text{eh}}(5'7)G^{\text{he}}(7'5) & G^{\text{hh}}(5'7)G^{\text{hh}}(7'5) \\ G^{\text{ee}}(5'7)G^{\text{ee}}(7'5) & G^{\text{he}}(5'7)G^{\text{eh}}(7'5)\end{pmatrix}. \tag{60}
$$

The effective interactions obtained using $\tilde{\boldsymbol{K}}_0$ are drawn up to third order in Fig. 1. There are quite a few interesting observations to make. First, the (normal) diagonal components of $\boldsymbol{T}$ include a first-order term, whereas the diagrammatic expansion of the anomalous components begins at second order. Therefore, the $T$-matrix self-energy of Eq. (58) has no first-order off-diagonal terms. This is consistent with the fact that the total self-energy [see Eq. (34)] is the sum of the first-order Bogoliubov self-energy [see Eq. (33)] and the $T$-matrix self-energy [see Eq. (58)]. Also, note that, when one considers both the normal and anomalous components, the $T$-matrix approximation of Eq. (58) is not exact up to second order. Figure 2 shows the self-energy diagrams up to second order in the Coulomb interaction [6]. The second-order terms included in the $T$-matrix of Eq. (58) correspond to the upper panel of Fig. 2. In Sec. VI, we show that the missing second-order terms (see lower panel) come up through the first vertex correction to the self-energy.

All terms of $T^{\text{hh}}$ and $T^{\text{ee}}$ involve at least one anomalous propagator. Therefore, these effective interactions vanish when the pairing field is switched off. Finally, this generalized effective interaction and the associated self-energies reduce exactly to the generalized $T$-matrix approximation introduced by Bozek to describe superfluid nuclear matter [8]. While this is likely a formidable task in practice, this formalism theoretically allows for the inclusion of vertex corrections in Bozek's approximation.

Before concluding this section, we report the Dyson equations of $\tilde{\boldsymbol{\Gamma}}^{\text{hh}}$ and $\tilde{\boldsymbol{\Gamma}}^{\text{ee}}$ that are derived using chain rules with respect to the propagators

$$
\begin{aligned}
\tilde{\boldsymbol{\Gamma}}^{\text{hh}}(44';3'1') &= \frac{1}{2}\begin{pmatrix} 0 & \delta(3'4)\delta(1'4')-\delta(3'4')\delta(1'4) \\ 0 & 0\end{pmatrix} + \frac{\delta\boldsymbol{\Sigma}(3'1')}{\delta V^{\text{hh}}(44')} \\
&= \tilde{\boldsymbol{\Gamma}}_0^{\text{hh}}(44';3'1') \\
&+ \frac{\delta\boldsymbol{\Sigma}(3'1')}{\delta G^{\text{he}}(55')}[\boldsymbol{G}(56)\tilde{\boldsymbol{\Gamma}}^{\text{hh}}(44';66')\boldsymbol{G}(6'5')]^{\text{he}} + \frac{\delta\boldsymbol{\Sigma}(3'1')}{\delta G^{\text{hh}}(55')}[\boldsymbol{G}(56)\tilde{\boldsymbol{\Gamma}}^{\text{hh}}(44';66')\boldsymbol{G}(6'5')]^{\text{hh}} \\
&+ \frac{\delta\boldsymbol{\Sigma}(3'1')}{\delta G^{\text{ee}}(55')}[\boldsymbol{G}(56)\tilde{\boldsymbol{\Gamma}}^{\text{hh}}(44';66')\boldsymbol{G}(6'5')]^{\text{ee}} + \frac{\delta\boldsymbol{\Sigma}(3'1')}{\delta G^{\text{eh}}(55')}[\boldsymbol{G}(56)\tilde{\boldsymbol{\Gamma}}^{\text{hh}}(44';66')\boldsymbol{G}(6'5')]^{\text{eh}},
\end{aligned} \tag{61a}
$$

$$
\begin{aligned}
\tilde{\boldsymbol{\Gamma}}^{\text{ee}}(44';3'1') &= \frac{1}{2}\begin{pmatrix} 0 & 0 \\ \delta(3'4)\delta(1'4')-\delta(3'4')\delta(1'4) & 0\end{pmatrix} + \frac{\delta\boldsymbol{\Sigma}(3'1')}{\delta V^{\text{ee}}(44')} \\
&= \tilde{\boldsymbol{\Gamma}}_0^{\text{ee}}(44';3'1') \\
&+ \frac{\delta\boldsymbol{\Sigma}(3'1')}{\delta G^{\text{he}}(55')}[\boldsymbol{G}(56)\tilde{\boldsymbol{\Gamma}}^{\text{ee}}(44';66')\boldsymbol{G}(6'5')]^{\text{he}} + \frac{\delta\boldsymbol{\Sigma}(3'1')}{\delta G^{\text{hh}}(55')}[\boldsymbol{G}(56)\tilde{\boldsymbol{\Gamma}}^{\text{ee}}(44';66')\boldsymbol{G}(6'5')]^{\text{hh}} \\
&+ \frac{\delta\boldsymbol{\Sigma}(3'1')}{\delta G^{\text{ee}}(55')}[\boldsymbol{G}(56)\tilde{\boldsymbol{\Gamma}}^{\text{ee}}(44';66')\boldsymbol{G}(6'5')]^{\text{ee}} + \frac{\delta\boldsymbol{\Sigma}(3'1')}{\delta G^{\text{eh}}(55')}[\boldsymbol{G}(56)\tilde{\boldsymbol{\Gamma}}^{\text{ee}}(44';66')\boldsymbol{G}(6'5')]^{\text{eh}}.
\end{aligned} \tag{61b}
$$

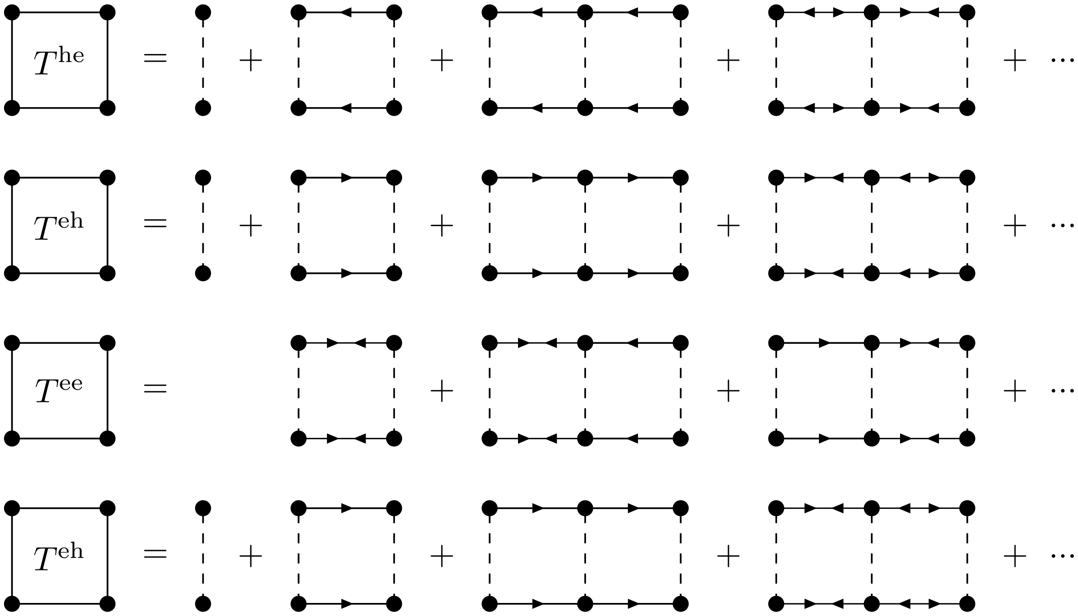


FIG. 1. The effective interaction $\boldsymbol{T}$ computed with the lowest-order vertex approximation results in a resummation of ladder diagrams for each component. The exchange counterpart of each of these diagrams should also be included but is not represented here. The double-arrowed propagators in $T^{\rm hh}$ ($T^{\rm ee}$) represent $G^{\rm hh}$ ($G^{\rm ee}$) [9].

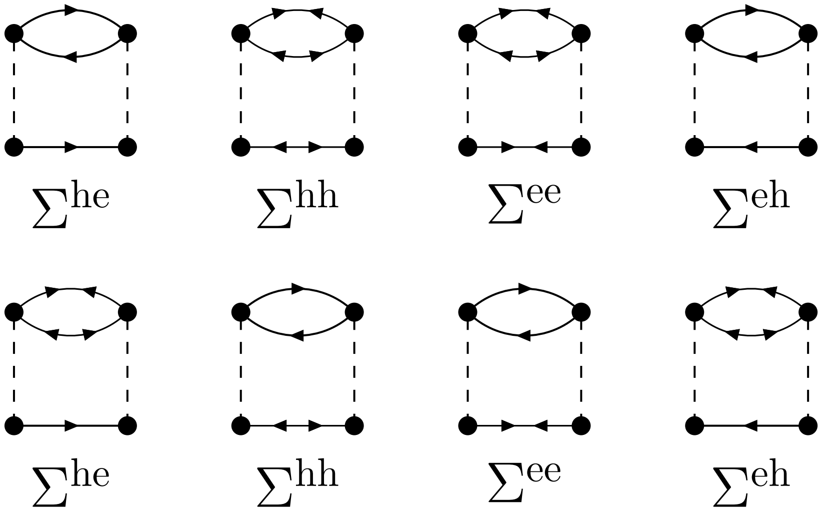


FIG. 2. The second-order terms of each component of $\boldsymbol{\Sigma}$. The exchange counterpart of each of these diagrams should also be included but is not represented here. The diagrams in the top row are included in the self-energy of first order in $\boldsymbol{T}$ [see Eq. (58)] while the diagrams in the bottom row come from the lowest-order vertex correction [see Eq. (74)].

## V. PARTICLE-PARTICLE HEDIN'S EQUATIONS

The aim of this section is to derive the set of equations of interest for number-conserving Hamiltonians. This is done by switching off the pairing potential ($U \to 0$), *i.e.* in the limit of vanishing pairing propagators. We remind the reader that $G^{\rm he}$ is the normal propagator. We will thus focus our attention on the upper-left block of the Gorkov-Dyson equation. In addition, we will also redefine some quantities in order to highlight the analogy with the original Hedin equations.

First, the Dyson equation remains unchanged and reads

$$G(11') = G_0(11') + G_0(12)\Sigma(22')G(2'1'), \tag{62}$$

while the self-energy of Eq. (49) becomes

$$\Sigma_{\text{Hxc}}(11') = \text{i}G(2'2^{++})T(12;33')\tilde{\Gamma}(33';2'1'), \tag{63}$$

where we removed the he superscript on $G$, $\Sigma$ and $T$ as the anomalous components are now zero. This expression is very similar to the $GW\Gamma$ expression of Hedin's equation, though with one notable difference which is that $GT\Gamma$ accounts for Hartree-exchange-correlation effects while the former is an exchange-correlation self-energy. The effective interaction $T$ in the normal phase admits the following Dyson equation

$$T(12;1'2') = -\bar{v}(12;1'2') - T(12;33')\tilde{K}(33';44')v(44'^{+};1'2'^{++}), \tag{64}$$

where the kernel is

$$\tilde{K}(12;1'2') = \text{i}\left.\frac{\delta G^{\text{ee}}(1'2')}{\delta V^{\text{ee}}(12)}\right|_{U=0} = \text{i}G(31')G(3'2')\tilde{\Gamma}(12;33'). \tag{65}$$

The missing ingredient is the vertex function

$$\tilde{\Gamma}(12;1'2') = \frac{\delta(G^{-1})^{\text{ee}}(1'2')}{\delta V^{\text{ee}}(12)} = \frac{1}{2}[\delta(1'2)\delta(2'1) - \delta(1'1)\delta(2'2)] - \Xi^{\text{pp}}(33';1'2')G(43)G(4'3')\tilde{\Gamma}(12;44'), \tag{66}$$

where the pp kernel is defined as

$$\Xi^{\text{pp}}(12;1'2') = \left.\frac{\delta\Sigma^{\text{ee}}(1'2')}{\delta G^{\text{ee}}(12)}\right|_{U=0}. \tag{67}$$

It is clear from this last definition that these five equations actually do not form a closed set of equations. Hence, in order to obtain vertex corrections, one first needs to iterate the closed set of equations for $\boldsymbol{G}$ (see Sec. IV) and, then, take the limit where the pairing propagators vanish. This will be done in Sec. VI. However, at the present stage, one can already study the effect of the lowest-order vertex approximation $\tilde{\Gamma}(12;1'2') = \frac{1}{2}[\delta(1'2)\delta(2'1) - \delta(1'1)\delta(2'2)]$ as the pp kernel naturally vanishes.

The corresponding self-energy reads

$$\Sigma(11') = \text{i}G(2'2)T(12;1'2'), \tag{68}$$

with the effective interaction

$$T(12;1'2') = -\bar{v}(12;1'2') - T(12;33')K_0(33';44')v(44'^{+};1'2'^{++}), \tag{69}$$

and

$$K_0(12;1'2') = \frac{\text{i}}{2}[G(12')G(21') - G(22')G(11')]. \tag{70}$$

Hence, the resulting approximation is exactly the $T$-matrix approximation computed at the pp-RPA level.

## VI. VERTEX CORRECTIONS TO THE $T$-MATRIX SELF-ENERGY

The aim of this last section is to derive the vertex corrections to the approximations derived previously in Secs. IV and V. As mentioned earlier, the derivation is first performed in the presence of a pairing potential and the normal-phase expressions are recovered in a second stage by taking the limit of a vanishing pairing potential. The first vertex correction is obtained by inserting Eqs. (59a) and (59b) into the Dyson equations for $\tilde{\boldsymbol{\Gamma}}^{\text{hh}}$ and $\tilde{\boldsymbol{\Gamma}}^{\text{ee}}$ [see Eqs. (61a) and

(61b)]

$$\begin{aligned}\tilde{\mathbf{\Gamma}}^{\mathrm{hh}}(44';3'1') =&\tilde{\mathbf{\Gamma}}_0^{\mathrm{hh}}(44';3'1') + \frac{1}{2}[\delta(46)\delta(4'6') - \delta(46')\delta(4'6)] \\ &\times\left\{\frac{\delta\mathbf{\Sigma}(3'1')}{\delta G^{\mathrm{he}}(55')}G^{\mathrm{he}}(56)G^{\mathrm{ee}}(6'5') + \frac{\delta\mathbf{\Sigma}(3'1')}{\delta G^{\mathrm{hh}}(55')}G^{\mathrm{he}}(56)G^{\mathrm{eh}}(6'5')\right. \\ &\left.+\frac{\delta\mathbf{\Sigma}(3'1')}{\delta G^{\mathrm{ee}}(55')}G^{\mathrm{ee}}(56)G^{\mathrm{ee}}(6'5') + \frac{\delta\mathbf{\Sigma}(3'1')}{\delta G^{\mathrm{eh}}(55')}G^{\mathrm{ee}}(56)G^{\mathrm{eh}}(6'5')\right\},\end{aligned} \tag{71a}$$

$$\begin{aligned}\tilde{\mathbf{\Gamma}}^{\mathrm{ee}}(44';3'1') =&\tilde{\mathbf{\Gamma}}_0^{\mathrm{ee}}(44';3'1') + \frac{1}{2}[\delta(46)\delta(4'6') - \delta(46')\delta(4'6)] \\ &\times\left\{\frac{\delta\mathbf{\Sigma}(3'1')}{\delta G^{\mathrm{he}}(55')}G^{\mathrm{hh}}(56)G^{\mathrm{he}}(6'5') + \frac{\delta\mathbf{\Sigma}(3'1')}{\delta G^{\mathrm{hh}}(55')}G^{\mathrm{hh}}(56)G^{\mathrm{hh}}(6'5')\right. \\ &\left.+\frac{\delta\mathbf{\Sigma}(3'1')}{\delta G^{\mathrm{ee}}(55')}G^{\mathrm{eh}}(56)G^{\mathrm{he}}(6'5') + \frac{\delta\mathbf{\Sigma}(3'1')}{\delta G^{\mathrm{eh}}(55')}G^{\mathrm{eh}}(56)G^{\mathrm{hh}}(6'5')\right\},\end{aligned} \tag{71b}$$

and then inserting into them Eq. (58). First, to investigate the expansion of $\tilde{\mathbf{\Gamma}}^{\mathrm{hh}}$ and $\tilde{\mathbf{\Gamma}}^{\mathrm{ee}}$, we neglect the terms involving derivatives of $T$. This is justified from a perturbative point of view as the derivative of the effective interaction with respect to $G$ is of second order in $T$. Focussing solely on the first-order terms simplifies the evaluation of these vertex functions

$$\begin{aligned}&\tilde{\mathbf{\Gamma}}^{\mathrm{hh}}(44';3'1') = \tilde{\mathbf{\Gamma}}_0^{\mathrm{hh}}(44';3'1') + \frac{1}{2}[\delta(46)\delta(4'6') - \delta(46')\delta(4'6)]\begin{pmatrix}\frac{\delta\Sigma^{\mathrm{he}}(3'1')}{\delta G^{\mathrm{eh}}(55')}G^{\mathrm{ee}}(56)G^{\mathrm{eh}}(6'5') & \frac{\delta\Sigma^{\mathrm{hh}}(3'1')}{\delta G^{\mathrm{ee}}(55')}G^{\mathrm{ee}}(56)G^{\mathrm{ee}}(6'5') \\ \frac{\delta\Sigma^{\mathrm{ee}}(3'1')}{\delta G^{\mathrm{hh}}(55')}G^{\mathrm{he}}(56)G^{\mathrm{eh}}(6'5') & \frac{\delta\Sigma^{\mathrm{eh}}(3'1')}{\delta G^{\mathrm{he}}(55')}G^{\mathrm{he}}(56)G^{\mathrm{ee}}(6'5')\end{pmatrix} \\ &= \tilde{\mathbf{\Gamma}}_0^{\mathrm{hh}}(44';3'1') + \frac{1}{2}[\delta(46)\delta(4'6') - \delta(46')\delta(4'6)] \\ &\times\begin{pmatrix}\frac{\delta G^{\mathrm{eh}}(77')}{\delta G^{\mathrm{eh}}(55')}T^{\mathrm{he}}(3'7;7'1')G^{\mathrm{ee}}(56)G^{\mathrm{eh}}(6'5') & \frac{\delta G^{\mathrm{ee}}(77')}{\delta G^{\mathrm{ee}}(55')}T^{\mathrm{hh}}(3'7;7'1')G^{\mathrm{ee}}(56)G^{\mathrm{ee}}(6'5') \\ \frac{\delta G^{\mathrm{hh}}(77')}{\delta G^{\mathrm{hh}}(55')}T^{\mathrm{ee}}(3'7;7'1')G^{\mathrm{he}}(56)G^{\mathrm{eh}}(6'5') & \frac{\delta G^{\mathrm{he}}(77')}{\delta G^{\mathrm{he}}(55')}T^{\mathrm{eh}}(3'7;7'1')G^{\mathrm{he}}(56)G^{\mathrm{ee}}(6'5')\end{pmatrix} \\ &= \tilde{\mathbf{\Gamma}}_0^{\mathrm{hh}}(44';3'1') + \frac{1}{2}[\delta(46)\delta(4'6') - \delta(46')\delta(4'6)] \\ &\times\begin{pmatrix}T^{\mathrm{he}}(3'7;7'1')G^{\mathrm{ee}}(76)G^{\mathrm{eh}}(6'7') & \frac{T^{\mathrm{hh}}(3'7;7'1')}{2}[G^{\mathrm{ee}}(76)G^{\mathrm{ee}}(6'7') - G^{\mathrm{ee}}(7'6)G^{\mathrm{ee}}(6'7)] \\ \frac{T^{\mathrm{ee}}(3'7;7'1')}{2}[G^{\mathrm{he}}(76)G^{\mathrm{eh}}(6'7') - G^{\mathrm{he}}(7'6)G^{\mathrm{eh}}(6'7)] & T^{\mathrm{eh}}(3'7;7'1')G^{\mathrm{he}}(76)G^{\mathrm{ee}}(6'7')\end{pmatrix},\end{aligned} \tag{72a}$$

$$\begin{aligned}&\tilde{\mathbf{\Gamma}}^{\mathrm{ee}}(44';3'1') = \tilde{\mathbf{\Gamma}}_0^{\mathrm{ee}}(44';3'1') + \frac{1}{2}[\delta(46)\delta(4'6') - \delta(46')\delta(4'6)]\begin{pmatrix}\frac{\delta\Sigma^{\mathrm{he}}(3'1')}{\delta G^{\mathrm{eh}}(55')}G^{\mathrm{eh}}(56)G^{\mathrm{hh}}(6'5') & \frac{\delta\Sigma^{\mathrm{hh}}(3'1')}{\delta G^{\mathrm{ee}}(55')}G^{\mathrm{eh}}(56)G^{\mathrm{he}}(6'5') \\ \frac{\delta\Sigma^{\mathrm{ee}}(3'1')}{\delta G^{\mathrm{hh}}(55')}G^{\mathrm{hh}}(56)G^{\mathrm{hh}}(6'5') & \frac{\delta\Sigma^{\mathrm{eh}}(3'1')}{\delta G^{\mathrm{he}}(55')}G^{\mathrm{hh}}(56)G^{\mathrm{he}}(6'5')\end{pmatrix} \\ &= \tilde{\mathbf{\Gamma}}_0^{\mathrm{ee}}(44';3'1') + \frac{1}{2}[\delta(46)\delta(4'6') - \delta(46')\delta(4'6)] \\ &\times\begin{pmatrix}\frac{\delta G^{\mathrm{eh}}(77')}{\delta G^{\mathrm{eh}}(55')}T^{\mathrm{he}}(3'7;7'1')G^{\mathrm{eh}}(56)G^{\mathrm{hh}}(6'5') & \frac{\delta G^{\mathrm{ee}}(77')}{\delta G^{\mathrm{ee}}(55')}T^{\mathrm{hh}}(3'7;7'1')G^{\mathrm{eh}}(56)G^{\mathrm{he}}(6'5') \\ \frac{\delta G^{\mathrm{hh}}(77')}{\delta G^{\mathrm{hh}}(55')}T^{\mathrm{ee}}(3'7;7'1')G^{\mathrm{hh}}(56)G^{\mathrm{hh}}(6'5') & \frac{\delta G^{\mathrm{he}}(77')}{\delta G^{\mathrm{he}}(55')}T^{\mathrm{eh}}(3'7;7'1')G^{\mathrm{hh}}(56)G^{\mathrm{he}}(6'5')\end{pmatrix} \\ &= \tilde{\mathbf{\Gamma}}_0^{\mathrm{ee}}(44';3'1') + \frac{1}{2}[\delta(46)\delta(4'6') - \delta(46')\delta(4'6)] \\ &\times\begin{pmatrix}T^{\mathrm{he}}(3'7;7'1')G^{\mathrm{eh}}(76)G^{\mathrm{hh}}(6'7') & \frac{T^{\mathrm{hh}}(3'7;7'1')}{2}[G^{\mathrm{eh}}(76)G^{\mathrm{he}}(6'7') - G^{\mathrm{eh}}(7'6)G^{\mathrm{he}}(6'7)] \\ \frac{T^{\mathrm{ee}}(3'7;7'1')}{2}[G^{\mathrm{hh}}(76)G^{\mathrm{hh}}(6'7') - G^{\mathrm{hh}}(7'6)G^{\mathrm{hh}}(6'7)] & T^{\mathrm{eh}}(3'7;7'1')G^{\mathrm{hh}}(76)G^{\mathrm{he}}(6'7')\end{pmatrix}.\end{aligned} \tag{72b}$$

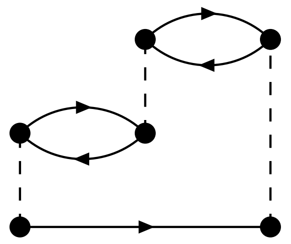

FIG. 3. A third-order self-energy term arising through the second iteration of the pp Hedin equations.

Note that, except for the zeroth-order terms $\tilde{\mathbf{\Gamma}}_0$, these vertex corrections are zero in the number-conserving limit. Therefore, there is no self-energy corrections at second order in $T$ in the normal phase. The next term of the expansion after Eq. (68) is of third order in the effective interaction. For the same reason, the lowest-order correction to $\tilde{K}$ in the normal phase is of second order in $T$.

Now, we would like to investigate the diagrammatic content of these corrections (in the presence of the pairing field). In particular, we show below that these vertex corrections incorporate the missing second-order terms in the Coulomb interaction $v$. Because the anomalous components of $T$ have no first-order terms, the self-energy has a non-zero second-order term in $v$ if and only if it is proportional to a single component of $\boldsymbol{T}$ or to a product of normal components, such as $T^{\text{he}}T^{\text{eh}}$. The former is included in Eq. (58) (top row of Fig. 2) and the latter comes from the vertex functions (bottom row of Fig. 2). To show this more explicitly, we compute the self-energy associated with the vertex functions derived above but keeping only the terms proportional to a product of normal components of $\boldsymbol{T}$. This gives

$$\begin{aligned}
&\frac{\mathrm{i}}{2}[\delta(46)\delta(4'6') - \delta(46')\delta(4'6)] \\
&\left[\begin{pmatrix} T^{\text{he}}(12;44') & 0 \\ 0 & 0 \end{pmatrix}\begin{pmatrix} G^{\text{ee}}(2^{++}3') & G^{\text{eh}}(2^{++}3') \\ G^{\text{he}}(2^{--}3') & G^{\text{hh}}(2^{--}3') \end{pmatrix}\begin{pmatrix} T^{\text{he}}(3'7;7'1')G^{\text{eh}}(76)G^{\text{hh}}(6'7') & 0 \\ 0 & T^{\text{eh}}(3'7;7'1')G^{\text{hh}}(76)G^{\text{he}}(6'7') \end{pmatrix}\right. \\
&\left.+\begin{pmatrix} 0 & 0 \\ 0 & T^{\text{eh}}(12;44') \end{pmatrix}\begin{pmatrix} G^{\text{ee}}(2^{++}3') & G^{\text{eh}}(2^{++}3') \\ G^{\text{he}}(2^{--}3') & G^{\text{hh}}(2^{--}3') \end{pmatrix}\begin{pmatrix} T^{\text{he}}(3'7;7'1')G^{\text{ee}}(76)G^{\text{eh}}(6'7') & 0 \\ 0 & T^{\text{eh}}(3'7;7'1')G^{\text{he}}(76)G^{\text{ee}}(6'7') \end{pmatrix}\right],
\end{aligned} \tag{73}$$

which can be recast as

$$\mathrm{i}\begin{pmatrix} T^{\text{he}}(12;66')G^{\text{ee}}(2^{++}3')T^{\text{he}}(3'7;7'1')G^{\text{eh}}(76)G^{\text{hh}}(6'7') & T^{\text{he}}(12;66')G^{\text{eh}}(2^{++}3')T^{\text{eh}}(3'7;7'1')G^{\text{hh}}(76)G^{\text{he}}(6'7') \\ T^{\text{eh}}(12;66')G^{\text{he}}(2^{--}3')T^{\text{he}}(3'7;7'1')G^{\text{ee}}(76)G^{\text{eh}}(6'7') & T^{\text{eh}}(12;66')G^{\text{hh}}(2^{--}3')T^{\text{eh}}(3'7;7'1')G^{\text{he}}(76)G^{\text{ee}}(6'7') \end{pmatrix}. \tag{74}$$

The second-order terms are obtained by replacing the effective interactions with the Coulomb interaction. They are represented in the lower panel of Fig. 2. Hence, after the first vertex corrections, the self-energy is now exact up to second order in the Coulomb interaction. It is worth mentioning that the $\Sigma^{\text{he}}$ component of Eq. (74) vanishes in the normal phase. We recover the well-known fact that the pp-RPA $T$-matrix is exact up to second order in $v$.

To conclude this study, the next iteration of the pp Gorkov-Hedin equations is partially performed. Our aim is to show that this also generates self-energy terms that are non-zero in the normal phase. This can be done by substituting the first-iteration self-energy of Eq. (74) into Eq. (66) to generate a new irreducible vertex. Here, we consider only the part of the vertex due to the first-iteration self-energy and the lowest-order irreducible vertex [see Eq. (57)], that is, the last term in the right-hand side of Eq. (66) is approximated as

$$\left.\frac{\delta\Sigma^{\text{ee}}(2'1')}{\delta G^{\text{ee}}(44')}\right|_{U=0} G^{\text{he}}(54)G^{\text{he}}(5'4')\frac{1}{2}[\delta(53')\delta(5'3) - \delta(53)\delta(5'3')], \tag{75}$$

where the ee component of the self-energy obtained in the previous iteration is given by

$$\Sigma^{\text{ee}}(2'1') = \mathrm{i}T^{\text{eh}}(2'8;66')G^{\text{he}}(8^{--}8')T^{\text{he}}(8'7;7'1')G^{\text{ee}}(76)G^{\text{eh}}(6'7'). \tag{76}$$

Hence, Eq. (75) becomes

$$\begin{aligned}
&\mathrm{i}T^{\text{eh}}(2'8;66')G^{\text{he}}(8^{--}8')T^{\text{he}}(8'7;7'1')G^{\text{eh}}(6'7')\left.\frac{\delta G^{\text{ee}}(76)}{\delta G^{\text{ee}}(44')}\right|_{U=0}\frac{1}{2}[G^{\text{he}}(3'4)G^{\text{he}}(34') - G^{\text{he}}(34)G^{\text{he}}(3'4')] \\
&\qquad = \mathrm{i}T^{\text{eh}}(2'8;66')G^{\text{he}}(8^{--}8')T^{\text{he}}(8'7;7'1')G^{\text{eh}}(6'7')\frac{1}{2}[G^{\text{he}}(3'7)G^{\text{he}}(36) - G^{\text{he}}(37)G^{\text{he}}(3'6)].
\end{aligned} \tag{77}$$

The self-energy term corresponding to this irreducible vertex reads [see Eq. (63)]

$$\mathrm{i}^2 G^{\mathrm{he}}(2'2^{++})T^{\mathrm{he}}(12;33')T^{\mathrm{eh}}(2'8;66')G^{\mathrm{he}}(8^{--}8')T^{\mathrm{he}}(8'7;7'1')G^{\mathrm{eh}}(6'7')G^{\mathrm{he}}(3'7)G^{\mathrm{he}}(36). \tag{78}$$

In terms of the Coulomb interaction, the lowest-order term of this approximation is of third order. The corresponding diagram is drawn in Fig. 3. Hence, the self-energy of Eq. (78) corresponds to the third-order $GW$ bubble diagram where the Coulomb interaction has been replaced by the effective interaction $T$. This is fully analog to the screened ladder diagrams that arise through the vertex corrections to the $GW$ self-energy in conventional Hedin's equations.

## ACKNOWLEDGMENTS

This project has received funding from the European Research Council (ERC) under the European Union's Horizon 2020 research and innovation programme (Grant agreement No. 863481).

[1] P. C. Martin and J. Schwinger, Theory of Many-Particle Systems. I, Phys. Rev. **115**, 1342 (1959).
[2] R. M. Martin, L. Reining, and D. M. Ceperley, *Interacting Electrons: Theory and Computational Approaches* (Cambridge University Press, 2016).
[3] H. van Aggelen, Y. Yang, and W. Yang, Exchange-correlation energy from pairing matrix fluctuation and the particle-particle random-phase approximation, Phys. Rev. A **88**, 030501 (2013).
[4] A. Marie, A. Ammar, and P.-F. Loos, The $GW$ Approximation: A Quantum Chemistry Perspective (2023), arxiv:2311.05351.
[5] F. Essenberger, *Density Functional Theory for Superconductors: Extension to a Pairing Mediated by Spin-Fluctuations*, Ph.D. thesis, Max Planck Institute of Microstructure Physics (2014).
[6] V. Somà, T. Duguet, and C. Barbieri, Ab initio self-consistent Gorkov-Green's function calculations of semimagic nuclei: Formalism at second order with a two-nucleon interaction, Phys. Rev. C **84**, 064317 (2011).
[7] T. Gál, The mathematics of functional differentiation under conservation constraint, J. Math. Chem. **42**, 661 (2007).
[8] P. Bożek, In medium T matrix for superfluid nuclear matter, Phys. Rev. C **65**, 034327 (2002).
[9] J.-P. Blaizot and G. Ripka, *Quantum Theory of Finite Systems* (The MIT Press, 1986).
